# Supplementary material for: Bonsai: Interpretable Tree-Adaptive Grounded Reasoning
Source: arXiv:2504.03640 source file (2025-04-04)
Supplement: Supplementary file 1 [file eqns.tex]

\section{Equations}

\begin{equation}
n= \begin{cases} 
      k_1 & x\leq m_1 \\
      \ceil{k_1+(x-m_2)} & m_1\leq x\leq m_2 \\
      \frac{100-x}{100} & m_2\leq x\leq m_3 \\
      k_3 & m_3\leq x 
   \end{cases}

\end{equation}
